# Supplementary material for: Bayesian optimization for inverse problems in time-dependent quantum dynamics
Source: arXiv:2006.06212 ancillary file (2020-08-14)
Supplement: Supplementary file 1 [file supplementary-information.pdf]

# Supplementary Information for "Bayesian optimization for inverse problems in time-dependent quantum dynamics"

Z. Deng[a], I. Tutunnikov[b], I. Sh. Averbukh[b], M. Thachuk[a], and R. V. Krems[a]
[a]*Department of Chemistry, University of British Columbia, Vancouver, B.C. V6T 1Z1, Canada*
[b]*AMOS and Department of Chemical and Biological Physics,*
*The Weizmann Institute of Science, Rehovot, 7610001, Israel*
(Dated: May 30, 2020)

Section I summarizes the calculated parameters used for producing the reference signals. The interaction potentials for the alignment and orientation simulations are provided in Sec. II. The impulsive approximation is described in Sec. III. Finally, Sec. IV contains the expressions for the observables, i.e. birefringence, and alignment and orientation factors.

## I. MOLECULAR PARAMETERS

Table I summarizes the reference molecular parameters for the two molecules used in this study.

($R$)-propylene oxide

| Mom. of inertia | Polarizability comp. | | Dipole comp. |
|---|---|---|---|
| $I_a = 180386$ | $\alpha_{aa} = 45.63$ | $\alpha_{ab} = 2.56$ | $d_a = 0.965$ |
| $I_b = 493185$ | $\alpha_{bb} = 37.96$ | $\alpha_{ac} = 0.85$ | $d_b = -1.733$ |
| $I_c = 553513$ | $\alpha_{cc} = 37.87$ | $\alpha_{bc} = 0.65$ | $d_c = 0.489$ |

Sulfur dioxide

| Mom. of inertia | Polarizability comp. | Dipole comp. |
|---|---|---|
| $I_a = 54106$ | $\alpha_{aa} = 31.26$ | $d_a = 0$ |
| $I_b = 318791$ | $\alpha_{bb} = 20.80$ | $d_b = -2.003$ |
| $I_c = 373860$ | $\alpha_{cc} = 18.64$ | $d_c = 0$ |

Supplementary Table I. Summary of molecular parameters expressed in the frame of principal axes of inertia tensor $a$, $b$ and $c$: moments of inertia (a.u.), polarizabilities (a.u.), and dipole components (Debye). For the chiral propylene oxide molecule, the provided values correspond to the right handed enantiomer ($R$).

In case of ($R$)-propylene oxide molecule [($R$)-PPO], the molecular parameters were obtained with the help of Gaussian software package [1] (method: CAM-B3LYP/augcc-pVTZ). Moments of inertia of the $SO_2$ molecule are from the experimental data provided on the NIST website [2], while its calculated polarizability and dipole moment are from Ref. [3].

## II. INTERACTION POTENTIALS

In the laboratory $XYZ$ frame, the angular momentum quantization axis is the $Z$ axis. Interaction potential for the case of a chiral molecule interacting with a $Z$-polarized electric field $\mathbf{E}(t) = \varepsilon(t)(0,0,1)^T$ can be written in terms of Wigner D-functions [4]

$$U(t) = -\frac{\varepsilon^2(t)}{2\sqrt{6}}\Big[D^{(2)*}_{0,-2}\alpha^{(2)}_{\mathrm{mol},-2} + D^{(2)*}_{0,-1}\alpha^{(2)}_{\mathrm{mol},-1} + D^{(2)*}_{0,0}\alpha^{(2)}_{\mathrm{mol},0} + D^{(2)*}_{0,1}\alpha^{(2)}_{\mathrm{mol},1} + D^{(2)*}_{0,2}\alpha^{(2)}_{\mathrm{mol},2}\Big], \quad (1)$$

where $\varepsilon(t)$ is the slowly varying envelope of the laser pulse, $D^{(r)*}_{p,q}$ are complex conjugated Wigner D-matrices [5], the $\alpha$-coefficients are the polarizabilities in the rotating molecular $xyz$ frame expressed in the spherical basis

$$\alpha^{(2)}_{\mathrm{mol},0} = \frac{1}{\sqrt{6}}(2\alpha_{zz} - \alpha_{xx} - \alpha_{yy})$$
$$\alpha^{(2)}_{\mathrm{mol},\pm1} = \mp(\alpha_{xz} \pm i\alpha_{yz})$$
$$\alpha^{(2)}_{\mathrm{mol},\pm2} = \frac{1}{2}(\alpha_{xx} - \alpha_{yy} \pm 2i\alpha_{xy}). \quad (2)$$

Interaction potential for the general case of a chiral molecule interacting with a linearly polarized in $XY$ plane electric field, $\mathbf{E}(t) = \varepsilon(t)(\cos\gamma, \sin\gamma, 0)^T$ is given by

$$U(t) = \frac{\varepsilon^2(t)}{8}\Big[\frac{2}{\sqrt{6}}D^{(2)*}_{0q}\alpha^{(2)}_{\mathrm{mol},q} - \Big(e^{2i\gamma}D^{(2)*}_{-2q}\alpha^{(2)}_{\mathrm{mol},q} + e^{-2i\gamma}D^{(2)*}_{2q}\alpha^{(2)}_{\mathrm{mol},q}\Big)\Big], \quad (3)$$

where $\gamma$ is the angle between the polarization direction and the $X$ axis. Summation over the index $q = -r, \ldots, r$ is implied (here, $r = 0, 2$). A derivation of the above expressions is outlined in Appendix to Ref. [6].

We define the following parameters $\alpha^{zx} = \alpha_{zz} - \alpha_{xx}$ and $\alpha^{zy} = \alpha_{zz} - \alpha_{yy}$, $\alpha_{xx} - \alpha_{yy} = \alpha^{zy} - \alpha^{zx}$ in terms of which the polarizabilities defined in Eq. 2 become

$$\alpha^{(2)}_{\mathrm{mol},0} = \frac{1}{\sqrt{6}}(\alpha^{zx} + \alpha^{zy})$$
$$\alpha^{(2)}_{\mathrm{mol},\pm1} = \mp\alpha_{xz} - i\alpha_{yz}$$
$$\alpha^{(2)}_{\mathrm{mol},\pm2} = \frac{1}{2}(\alpha^{zy} - \alpha^{zx} \pm 2i\alpha_{xy}). \quad (4)$$

By direct substitution and rearrangement it can be shown that the interaction potential depends on five parameters only, $\{\alpha^{zx}, \alpha^{zy}, \alpha_{xz}, \alpha_{yz}, \alpha_{xy}\}$. As expected, this holds true for the $Z$-polarized pulse as well. All the formulas can be applied to the case of non-chiral molecule (e.g. sulfur dioxide) as well, simply by setting the off-diagonal polarizability components to zero.

In our simulations at 0 K, the principal axes of inertia tensor of both sulfur dioxide and propylene oxide molecules are associated with the axes of the rotating frame according to $x \leftrightarrow b, y \leftrightarrow c, z \leftrightarrow a$.

In contrast, in our finite temperature simulations for sulfur dioxide, the assignment is $x \leftrightarrow a, y \leftrightarrow c, z \leftrightarrow b$. This choice is convenient for accounting for spin symmetry selection rules of the sulfur dioxide molecule. For this molecule, only rotational levels that are symmetric with respect to the $b$ axis were taken into account. Setting the $b$ axis along the $z$ axis of the rotating frame allows to consider only states with even $K$ quantum number.

## III. IMPULSIVE APPROXIMATION

In this study, we assume that the laser pulses are short in time as compared to the typical rotational period of a molecule at a given temperature, which justifies the so called "impulsive approximation". Under this approximation, the kinetic part of the Hamiltonian may be neglected during the operation of the laser pulse, and the full Hamiltonian can be approximated by $H \approx U$. The Shrödinger equation (in a.u.) becomes $i\mathrm{d}\psi/\mathrm{d}t = U\psi$, which can be solved by integration

$$i\int \frac{\mathrm{d}\psi}{\psi} = \int\limits_{-\infty}^{\infty} U\mathrm{d}t \iff i\ln\frac{\psi_+}{\psi_-} = \int\limits_{-\infty}^{\infty} U\mathrm{d}t.$$

Here, we denote the wave function just before the laser pulse by $\psi_-$ and just after it by $\psi_+$. For Gaussian laser pulses, the pulse envelope is given by $\varepsilon(t) = \varepsilon_0 e^{-2\ln 2(t/\tau)^2}$,where $\tau$ is the full width at half maximum of the *intensity* profile, and peak intensity $I_0 \equiv \varepsilon^2(t = 0) = \varepsilon_0^2$. The wave function just after the pulse is given by

$$\psi_+ = \psi_- \exp\left[\frac{i\tau I_0\sqrt{\pi/\ln 16}}{4}\tilde{U}\right].$$

where $\tilde{U} = U/\varepsilon^2(t)$.

To summarize, in addition to its dependence on $\{\alpha^{zx}, \alpha^{zy}, \alpha_{zx}, \alpha_{zy}, \alpha_{xy}\}$, the wave function also depends on the product of intensity and the width of the intensity profile, $\tau$. Notice, this holds true only within the impulsive approximation.

## IV. OBSERVABLES

In this study, we focus on two main observables. In case of sulfur dioxide, it is the birefringence

$$B(t) \propto \sum_{i=x,y,z} k_i \langle\cos^2(\theta_{iZ})\rangle, \tag{5}$$

where $k_z = \alpha^{zx} + \alpha^{zy}$, $k_x = -(2\alpha^{zx} + \alpha^{zy})$, $k_y = \alpha^{zx} - 2\alpha^{zy}$, $\alpha^{zx} = \alpha_{zz} - \alpha_{xx}$, $\alpha^{zy} = \alpha_{zz} - \alpha_{yy}$ and $\theta_{iZ}$ are the angles between the corresponding axes of the molecule fixed frame and the laser pulse (polarized along the $Z$ axis). The alignment factors with respect to the $Z$ axis are given by

$$\langle\cos^2(\theta_{iZ})\rangle = -\frac{1}{\sqrt{3}} A^{(0)}_{\mathrm{mol},0} D^{(0)}_{00} + \frac{2}{\sqrt{6}}\left[A^{(2)}_{\mathrm{mol},-2} D^{(2)}_{0,2} + A^{(2)}_{\mathrm{mol},0} D^{(2)}_{0,0} + A^{(2)}_{\mathrm{mol},2} D^{(2)}_{0,-2}\right], \tag{6}$$

where

$$A^{(0)}_{\mathrm{mol},0} = -\frac{1}{\sqrt{3}}\left(m_x^2 + m_y^2 + m_z^2\right)$$
$$A^{(2)}_{\mathrm{mol},0} = \frac{1}{\sqrt{6}}\left(2m_z^2 - m_x^2 - m_y^2\right)$$
$$A^{(2)}_{\mathrm{mol},\pm 2} = \frac{1}{2}\left(m_x^2 - m_y^2 \pm 2i m_x m_y\right).$$

For example, in case of alignment of the $z$ axis with respect to the $Z$ axis, $\langle\cos^2(\theta_{zZ})\rangle$ we set $m_x = m_y = 0$.

In the case of alignment of propylene oxide, the observable is the alignment factor of the molecular axis $a$ (which is close to the most polarizable axis of the molecule) with respect to the $Z$ axis $\langle\cos^2(\theta_{aZ})\rangle$ (see Eq. 6).

In the case of orientation of chiral propylene oxide molecule, the observable is the expectation value of projection of molecular dipole $\boldsymbol{\mu}$ on the laboratory $Z$ axis, $\mu_Z = \boldsymbol{\mu}\cdot\hat{\mathbf{Z}} = \mu\cos(\theta_{\mu Z})$, where $\mu = |\boldsymbol{\mu}|$ is the magnitude of the dipole moment, $\hat{\mathbf{Z}}$ is the unit vector along the $Z$ axis, and $\theta_{\mu Z}$ is the angle between the molecular dipole moment and the $Z$ axis. The observable can be expressed in terms of Wigner D-functions

$$\langle\mu_Z\rangle = \langle\psi|\sum_{q=-1}^{1} D^{(1)}_{0,q}\mu^{(1)}_{\mathrm{mol},q}|\psi\rangle,$$

where spherical tensor components of the molecular dipole are given in terms of Cartesian dipole components $\mu^{(1)}_{\mathrm{mol},\pm 1} = (\mp\mu_x - i\mu_y)/\sqrt{2}$ and $\mu^{(1)}_{\mathrm{mol},0} = \mu_z$.

Derivation of the above expressions is outlined in Appendix to Ref. [6].

[1] M. J. Frisch, G. W. Trucks, H. B. Schlegel, *et al.*, "Gaussian 16 Revision C.01," (2016), Gaussian Inc. Wallingford CT.

[2] G. Herzberg, *Electronic Spectra and Electronic Structure of Polyatomic Molecules*, Electronic Spectra and Electronic Structure of Polyatomic Molecules No. 2 (Krieger Publishing Company, 1991).

[3] G. Maroulis, *"The electric hyperpolarizability of ozone and sulfur dioxide,"* Chem. Phys. Lett **189**, 112 (1992).

[4] C. P. Koch, M. Lemeshko, and D. Sugny, *"Quantum control of molecular rotation,"* Rev. Mod. Phys. **91**, 035005 (2019).

[5] R. N. Zare, *Angular Momentum: Understanding Spatial Aspects in Chemistry and Physics* (Wiley-Interscience, 1991).

[6] I. Tutunnikov, J. Floß, E. Gershnabel, P. Brumer, and I. Sh. Averbukh, *"Laser-induced persistent orientation of chiral molecules,"* Phys. Rev. A **100**, 043406 (2019).
